# Supplementary material for: Intercalation-induced states at the Fermi level and the coupling of intercalated magnetic ions to conducting layers in Ni$_{1/3}$NbS$_2$
Source: arXiv:2401.05884 source file (2024-02-15)
Supplement: Supplementary file 1 [file reSupplemental-materials_NiNb3S6_YUtsumi6.pdf]

Supplemental materials to

# Intercalation-induced states at the Fermi level and the coupling of intercalated magnetic ions to conducting layers in $Ni_{1/3}NbS_2$

Yuki Utsumi Boucher[1], Izabela Biało[2, *], Mateusz A. Gala[2], Wojciech Tabiś[2], Marcin Rosmus[3, 4], Natalia Olszowska [3], Jacek J. Kolodziej[3, 4], Bruno Gudac[5], Mario Novak[5], Naveen Kumar Chogondahalli Muniraju[1, 6], Ivo Batistić[5], Neven Barišić[5, 7], Petar Popčević[1], and Eduard Tutiš[1]

[1] Institute of Physics, Bijenička c. 46, 10000 Zagreb, Croatia
[2] AGH University of Krakow, Faculty of Physics and Applied Computer Science, 30-059 Krakow, Poland
[3] Solaris National Synchrotron Radiation Centre, Jagiellonian University, Czerwone Maki 98, 30-392 Krakow, Poland
[4] Faculty of Physics, Astronomy, and Applied Computer Science, Jagiellonian University, Łojasiewicza 11, 30-348 Krakow, Poland
[5] Department of Physics, Faculty of Science, University of Zagreb, Bijenička c. 32, 10000 Zagreb, Croatia
[6] Institute of Nuclear Physics PAN, Radzikowskiego 152, 31-342 Kraków, Poland
[7] Institute of Solid State Physics, TU Wien, 1040 Vienna, Austria
[*] (current affiliation) Physik-Institut, Universität Zürich, Winterthurerstrasse 190, CH-8057 Zürich, Switzerland

## 1. Unfolding the electronic band structure of $Ni_{1/3}NbS_2$ into the first Brillouin zone of 2H-$NbS_2$

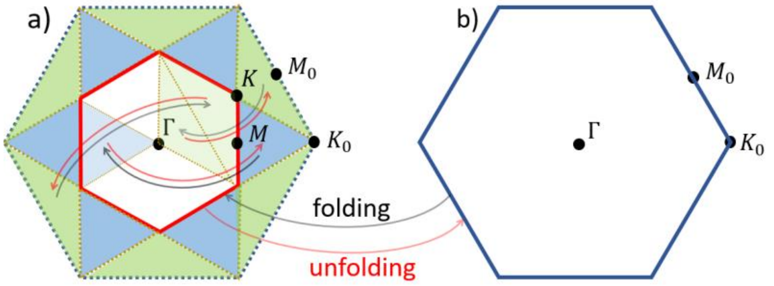


Fig. S1 The unfolding of the (small) first Brillouin zone of $Ni_{1/3}NbS_2$ into the (large) first Brillouin zone of 2H-$NbS_2$. a) The boundary of the projection of the first Brillouin zone of $Ni_{1/3}NbS_2$ in the $k_z = 0$ plane is shown as a white hexagon within a thick red border. The threefold bigger first Brillouin zone of 2H-$NbS_2$ is shown as the big hexagon shape in a blue dashed thick line. Upon unfolding, the three copies of the small white hexagon are needed to fill the big hexagon. The arrows illustrate the correspondence between parts

of the small white hexagon and the parts of the outer rim of the large hexagon. (b) The large first Brillouin zone of 2H- $NbS_2$ and its characteristic high symmetry points.

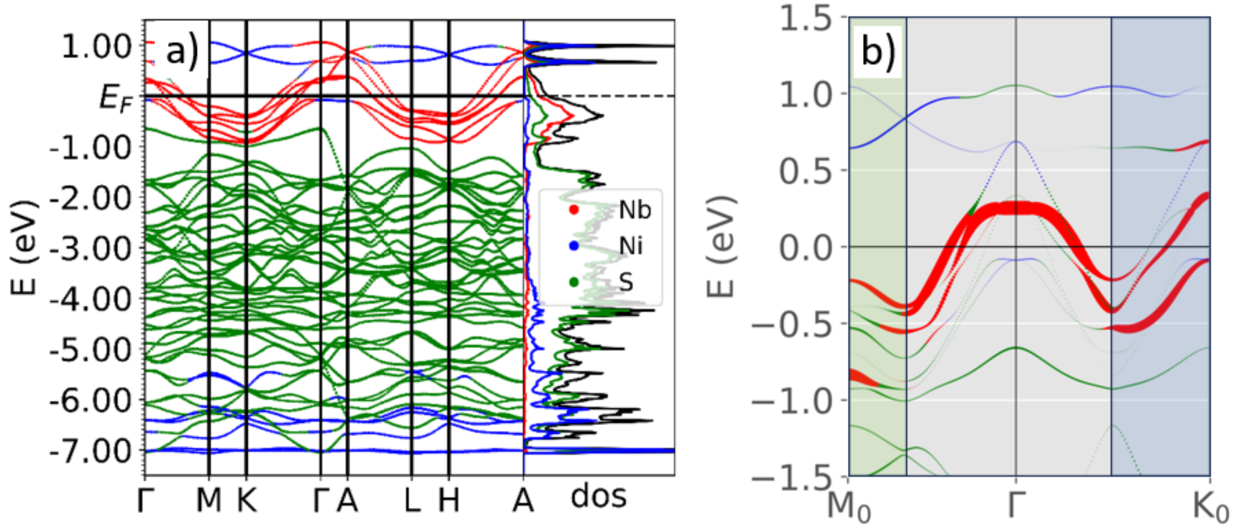


Fig. S2. (a) The electronic bands' dispersion and the density of states for $Ni_{1/3}NbS_2$ calculated in the antiferromagnetically ordered state. The colors on the dispersions plot indicate the types of atoms whose orbitals dominantly contribute to the corresponding electronic states. The same colors denote the partial density of states on the right panel, where the total density of states is shown in the black line. The projections are calculated from the corresponding orbital amplitudes of the wavefunction within the Wannier90 representation. The relaxation of the structure within the calculation produces the lattice constants of *a*= 5.73 Å and *c*= 11.86 Å, very comparable to experimental values. The labels correspond to the high symmetry points of the first Brillouin zone of $Ni_{1/3}NbS_2$. (b) The unfolded spectra along the $\overline{M_0\Gamma}$ and $\overline{\Gamma K_0}$ lines of Fig. S1(a). The same colors as in (a) are used to denote the dominant contribution of different atomic orbitals to the signal. The greenish and bluish rectangular shades denote the parts of the Brillouin zone shown in bluish and greenish shades in Fig. S1. The variation in intensity comes from the unfolding weights. In addition, the contributions from particular orbitals were multiplied by the photoionization intensities for Nb-4*d*, Ni-3*d*, and S-3*p* orbitals exposed to 40 eV photons [Yeh1985].

## 2. The effect of choosing different inner potential $V_0$ on the extracted spectrum

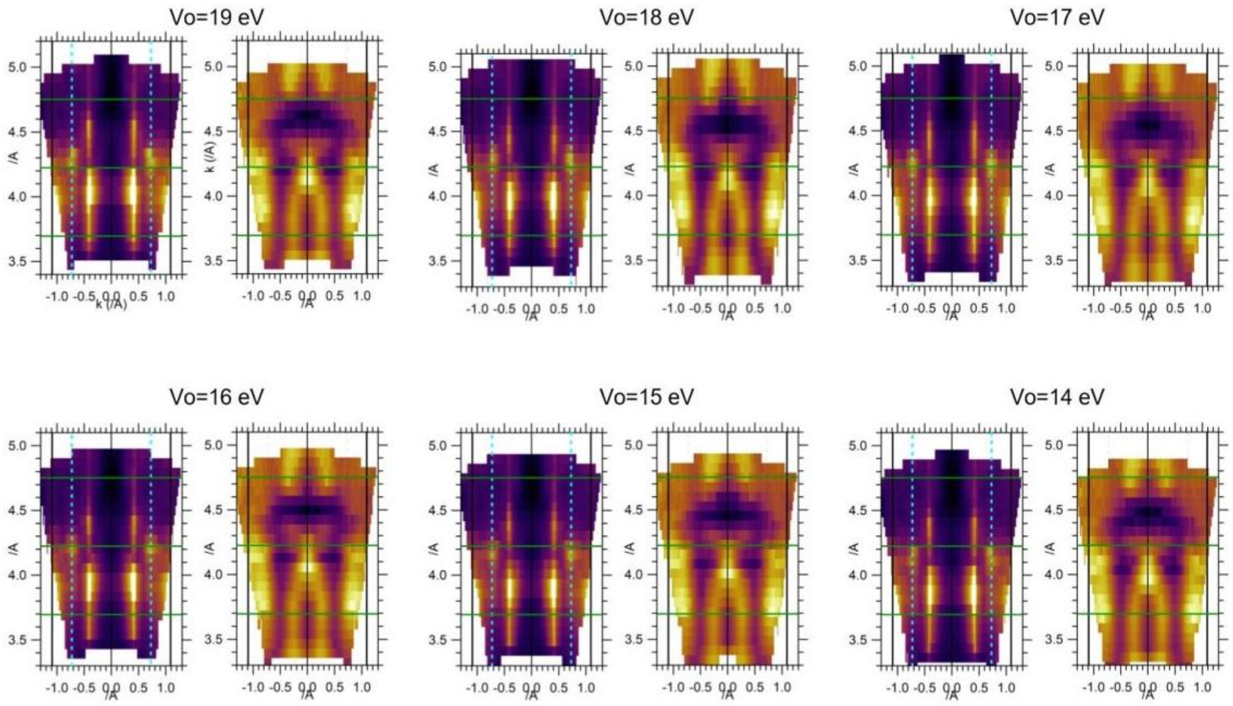


Fig. S3. The figure shows essentially the same spectrum as Fig. 3 in the paper. However, the extraction from the scanned data and the plots are performed here using different inner potential $V_0$ values. The change in the $V_0$ parameter changes the $k_z$ attributed to a particular data point, resulting in different $k_z$ spans for different $V_0$'s, changes in the vertical axes span, and slight differences in the images produced. The choice of $V_0 = 14$ eV is made for in Fig. 3 in the paper, earlier used in the sister compound $Cr_{1/3}NbS_2$ [Sirica2016]. Note, however, that the top surface layers of cleaved $Cr_{1/3}NbS_2$ and $Ni_{1/3}NbS_2$ systems are expected to have differently charged ions, similar to the difference between Co- and Ni-based systems mentioned in the main text, thus producing different surface dipole layers.

## 3. The Ni orbitals and their effective hybridization with Nb orbitals of the conduction bands

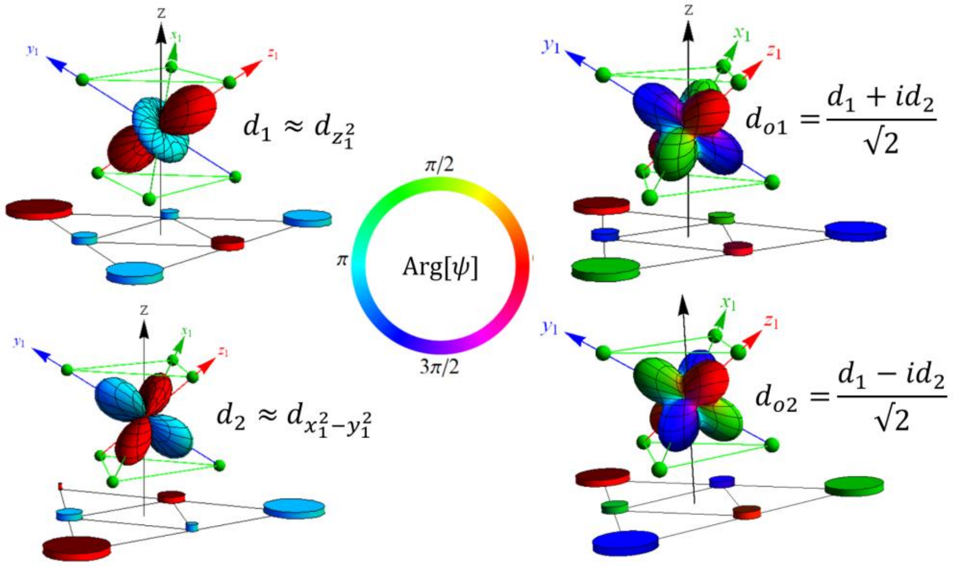


Fig. S4. The Ni orbitals with energy levels close to the Fermi level and with significant hybridization to Nb orbitals, which dominantly build the conduction bands in $NbS_2$ layers. Their energy levels are positioned approximately 0.69 eV above the Fermi level and 0.94 eV above the energy of the Nb orbitals in conduction bands. On the left, the two Ni 3$d$ $e_g$ orbitals, $d_1$, and $d_2$, are pictured, resembling closely the standard $d_{z_1^2}$ and $d_{x_1^2-y_1^2}$ orbitals, and extending along axes set by the sulfur octahedron. The cylinders below indicate the sizes and the complex signs (through their color) of the hybridization integrals to the nearby Nb orbitals in the layer below (same as in the main text). The color wheel for the complex phase of wavefunctions ($\psi = d_1, d_2, d_{o1}, d_{02}$) is shown in the center. Their linear combinations $d_{o1}$ and $d_{o2}$, conforming to the octahedral symmetry of the Ni surroundings, are shown on the right. The figure extends Fig. 5 of the main text, where more technical details are given regarding such plots.

## 4. The temperature dependence of the electrical resistivity of the $Ni_{1/3}NbS_2$ sample

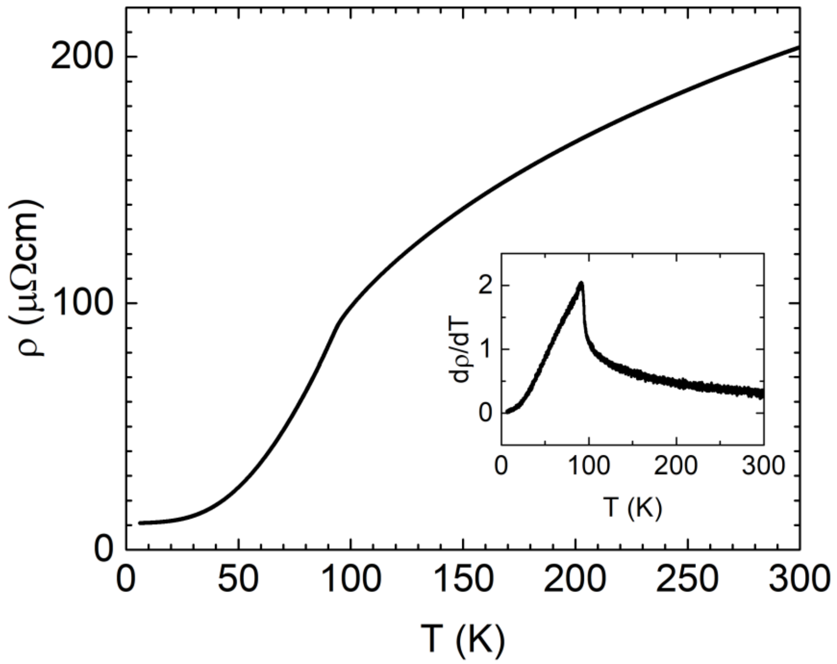


Fig. S5. Electrical resistivity measured on the sample from the same batch as the one used for the ARPES experiment. A sharp peak in the electrical resistivity derivative marks the position of the magnetic transition.

## References:


**[Sirica2016]:** N. Sirica, S.-K. Mo, F. Bondino, I. Pis, S. Nappini, P. Vilmercati, J. Yi, Z. Gai, P. C. Snijders, P. K. Das, I. Vobornik, N. Ghimire, M. R. Koehler, L. Li, D. Sapkota, D. S. Parker, D. G. Mandrus, and N. Mannella, Physical Review B **94**, 075141 (2016)

**[Yeh1985]** J.J. Yeh and I.Lindau, Atomic Data and Nuclear Data Tables, **32**, 1-155 (1985), also available through Ellectra synchrotron web site https://vuo.elettra.eu/services/elements/WebElements.html.
